# Supplementary material for: SPARK-Remote: A Cost-Effective System for Remote Bimanual Robot Teleoperation
Source: arXiv:2504.05488 source file (2025-04-29)
Supplement: Supplementary file 1 [file Appendix.tex]

\subsection{Hardware Design Details}

\subsection{Consumer Hardware}
\subsubsection{SpaceMouse} 
In this mode, we use two 3Dconnexion SpaceMouses, which are six-dimensional joystick controllers that provide three-dimensional translational $(x,y,z)$ and three-dimensional rotational $(\phi,\theta,\psi)$ information. Here, it functions as a speed controller, translating joystick values into movement rates. 
The gripper is controlled with two buttons to open and close it.

\subsubsection{VR Controllers}
In this mode, we use HTC Vive controllers and base stations to capture relative translations and rotations. When the menu button is pressed, $(x,y,z)$ translations are mirrored by the associated UR5e, and the grip button allows for rotational adjustments in $(\phi,\theta,\psi)$, and the trigger controls the gripper state. 
%This configuration enables the operator to adjust the end effector’s position and orientation comfortably. 

% , offering analog adjustments that only affect the gripper state when translating or rotating.

% \subsection{SpaceMouse}
% The 3Dconnexion SpaceMouse is a six-dimensional joystick that provides $x$/$y$/$z$ translational and roll/pitch/yaw information.
% Here, it functions as a speed controller, translating joystick values into movement rates. 
% The gripper is controlled with two buttons: one to fully open and another to fully close it.

%-------------------------------------------------------------------------

% \subsection{Ease of Use}
% \label{ease_of_use}
\subsection{Collision with Environment} 
\label{sec:collision}
SPARK is specifically designed to address challenges associated with bimanual teleoperation.
In single-arm teleoperation, the kinematic configuration is often less critical, as environmental collisions are minimized. However, with two arms, additional kinematic constraints introduce complexities that require attention \kar{elaborate?}. One common issue is self-collision, where parts of the manipulator’s structure collide with themselves or each other. This can happen if inverse kinematics generates a trajectory that causes a collision between the payload and the manipulator’s structure, a situation that typically requires modeling collision boundaries. SPARK bypasses this issue by avoiding Cartesian inverse kinematics, allowing the operator to directly select joint-level trajectories
A similar challenge arises with dual-arm interactions, where the kinematic structures of both arms can collide. For example, in the configuration shown in Figure \ref{fig:setup} \kar{TODO}, if both arms rotate toward each other, their elbow joints may collide. In smaller scales, wrist joints may also encounter configurations where inter-arm collisions prevent task completion. Navigating the robot's null-space in such cases can be unintuitive. While inverse kinematics could model and address these interactions, doing so limits the available solution space. Since the UR5e has only six degrees of freedom and is already prone to gimbal lock in its inverse kinematics, this could lead to problems with inverse kinematics.

\subsection{Gimbal Lock} 
\label{sec:gimbal_lock}
Gimbal lock is a significant challenge in our bimanual setup, where both UR5e manipulators have base joint axes positioned close to common end-effector positions.
As the end effector nears the line created by extending the base joint’s rotational axis, gimbal lock can occur, causing inverse kinematics to fail as the shoulder would need to rotate at ~\kar{missed something here}. Although more advanced inverse kinematics can mitigate gimbal lock, these methods often involve trade-offs in latency and computational load. Users may also find it non-intuitive to detect gimbal lock when using cartesian-based teleoperation systems. SPARK avoids this problem; users can feel when they approach gimbal lock and adjust accordingly. \kar{If policy learning is done at the joint level, this ability to navigate gimbal lock can also be embedded in the policy.}

% ------------------------------------------------

The UR5e robot is described using DH parameters, which define the transformation between consecutive links. The DH parameters are stored in \texttt{self.ur5e\_DH}:

\[
\text{DH Parameters} = \begin{bmatrix}
0 & 0 & 0.1625 & \frac{\pi}{2} \\
0 & -0.425 & 0 & 0 \\
0 & -0.3922 & 0 & 0 \\
0 & 0 & 0.1333 & \frac{\pi}{2} \\
0 & 0 & 0.0997 & -\frac{\pi}{2} \\
0 & 0 & 0.0996 & 0
\end{bmatrix}
\]

\section{Forward Kinematics}

The forward kinematics is computed using the DH parameters to obtain the transformation matrix \( T \):

\[
T = \prod_{j=1}^{6} A_j
\]

where \( A_j \) is the transformation matrix for joint \( j \):

\[
A_j = \begin{bmatrix}
\cos(\theta_j) & -\sin(\theta_j)\cos(\alpha_j) & \sin(\theta_j)\sin(\alpha_j) & a_j\cos(\theta_j) \\
\sin(\theta_j) & \cos(\theta_j)\cos(\alpha_j) & -\cos(\theta_j)\sin(\alpha_j) & a_j\sin(\theta_j) \\
0 & \sin(\alpha_j) & \cos(\alpha_j) & d_j \\
0 & 0 & 0 & 1
\end{bmatrix}
\]

\section{Loss Functions}

The total loss is a combination of the torque loss and the IK loss:

\subsection{Torque Loss}
The torque loss is computed as the sum of squared differences between the current joint angles (\(\theta\)) and the target torques (\(\text{targets}\)):

\[
\text{Torque Loss} = \sum_{i=1}^{6} (\theta_i - \text{targets}_i)^2
\]

\subsection{IK Loss}
The IK loss is computed as the squared difference between the end-effector position \( T_{2,3} \) and the desired position (0.6):

\[
\text{IK Loss} = (T_{2,3} - 0.6)^2 \times 100
\]

\subsection{SPARK Loss}
If SPARK control is enabled, the SPARK loss is computed as the sum of squared differences between the current joint angles (\(\theta\)) and the SPARK angles (\(\text{spark}\)):

\[
\text{SPARK Loss} = 2 \times \sum_{i=1}^{6} (\theta_i - \text{spark}_i)^2
\]

\section{Combined Loss}
The combined loss is a weighted sum of the torque loss and the SPARK loss, where the weights are determined by the torque and SPARK factors:

\[
\text{Loss} = \text{SPARK Loss} \times \text{spark} + \text{Torque Loss} \times \text{torque}
\]

where:

\[
\text{torque} = \frac{\max(\text{raw torques}) - \text{min torque}}{\text{max torque} - \text{min torque}}
\]

\[
\text{spark} = 1 - \text{torque}
\]

\section{Gradient Descent}

The gradients of the loss with respect to the joint angles (\(\theta\)) are computed using PyTorch's automatic differentiation. The joint angles are updated using gradient descent:

\[
\theta \leftarrow \theta - \eta \nabla_{\theta} \text{Loss}
\]

where \( \eta \) is the learning rate.

\section{Control Command}

The control command is computed as the mean of the gradients over a buffer of size 1:

\[
\text{command} = \frac{1}{\text{buf size}} \sum_{i=1}^{\text{buf size}} \text{grad}
\]

The command is then sent to the robot to control the joint velocities:

\[
\text{self.arms.speedJ(arm, [command, 6, 0.005])}
\]

\section{Summary}

% -----------------------

The SPARK joint angle control and force control work together to achieve smooth and precise movements of the UR5e robot. The combined loss function ensures that the joint angles are optimized to minimize torques while achieving the desired end-effector position. The gradients are computed using PyTorch's automatic differentiation, and the joint angles are updated using gradient descent. The control command is then sent to the robot to control the joint velocities.
